# Supplementary material for: A Tensor Network Implementation of Multi Agent Reinforcement Learning
Source: arXiv:2401.03896 source file (2024-01-08)
Supplement: Supplementary file 2 [file appendix2.tex]

\chapter{Mathematical Model of the Cavity - Emitter system}
